# Supplementary material for: Unveiling the Face-Dependent Ice Growth Kinetics: Insights from Molecular Dynamics on the Basal and Prism Surfaces
Source: arXiv:2410.07050 source file (2025-01-12)
Supplement: Supplementary file 1 [file SI.tex]

\title%[Sample title]
{SUPPLEMENTARY MATERIAL: Unveiling the Face-Dependent Ice Growth Kinetics: Insights from Molecular Dynamics on the Basal and Prism Surfaces}
% Force line breaks with \\
\author{Jihong Shi}
\affiliation{Department of Physics, King's College London, Strand, London WC2R 2LS, UK.%\\This line break forced% with \\
}
\author{Maxwell Fulford}
\affiliation{Department of Physics, King's College London, Strand, London WC2R 2LS, UK.%\\This line break forced% with \\
}
 %\altaffiliation[Also at ]{}%Lines break automatically or can be forced with \\
\author{Matteo Salvalaglio}
\affiliation{Department of Chemical Engineering, University College London, Torrington Place, London WC1E 7JE, UK.}

\author{Carla Molteni$^{\ast}$}
 \email{carla.molteni@kcl.ac.uk}
%\homepage{http://www.Second.institution.edu/~Charlie.Author.}
\affiliation{Department of Physics, King's College London, Strand, London WC2R 2LS, UK.%\\This line break forced% with \\
}

\date{\today}

\maketitle

%\begin{quotation}
%%%%%%%%%\end{quotation}
\begin{figure*}
%[htbp]
\centering
\includegraphics[width=1.0\textwidth]{FigS1.pdf}
\caption{(a) The initial and (b) the final structures in an 80 ns recrystallization simulation at 260 K for the basal surface. (c) The initial and (d) the final structures in a 70 ns recrystallization simulation at 260 K for the prism1 surface. The liquid-like molecules are coloured in red, and the ice-like molecules are in blue. Only oxygen atoms are shown.}
\label{melting_growth}
\end{figure*}

\begin{figure*}[htbp]
\centering
\includegraphics[width=1.1\textwidth]{FigS2.pdf}
\caption{(a) For the basal surface, the time-evolution of $\Delta n_l$ during the TIP4P/Ice crystallization simulations for one replica at each simulated temperature and (b) for the prism1 surface. (c) For the basal surface, the time-evolution of $\Delta n_l$ during the mW crystallization simulations for one replica at each simulated temperature and (d) for the prism1 surface.}
\label{envolution}
\end{figure*}

\begin{figure*}[htbp!]
\centering
\includegraphics[width=0.495\textwidth]{FigS3a.pdf}
\includegraphics[width=0.495\textwidth]{FigS3b.pdf}
\caption{Time-evolution of the excess number of liquid-like molecules $\Delta n_l$ during the TIP4P/Ice crystallization simulations three replicas of the ice Ih basal (left panel) and prism1 (right panel) surfaces at 240 K. The piecewise linear fitting technique obtained the ice growth rate. The liquid-like molecules were evaluated using order parameter $lq_3$ with a threshold of -0.67.}
\label{240K}
\end{figure*}

\begin{figure*}[htbp!]
\centering
\includegraphics[width=0.495\textwidth]{FigS4a.pdf}
\includegraphics[width=0.495\textwidth]{FigS4b.pdf}
\caption{Time-evolution of the excess number of liquid-like molecules $\Delta n_l$ during the TIP4P/Ice crystallization simulations three replicas of the ice Ih basal (left panel) and prism1 (right panel) surfaces at 245 K. The piecewise linear fitting technique obtained the ice growth rate. The liquid-like molecules were evaluated using order parameter $lq_3$ at a threshold of -0.67.}
\label{245k}
\end{figure*}

\begin{figure*}[htbp!]
\centering
\includegraphics[width=0.495\textwidth]{FigS5a.pdf}
\includegraphics[width=0.495\textwidth]{FigS5b.pdf}
\caption{Time-evolution of the excess number of liquid-like molecules $\Delta n_l$ during the TIP4P/Ice crystallization simulations three replicas of the ice Ih basal (left panel) and prism1 (right panel) surfaces at 250 K. The piecewise linear fitting technique obtained the ice growth rate. The liquid-like molecules were evaluated using order parameter $lq_3$ at a threshold of -0.67.}
\label{250k}
\end{figure*}

\begin{figure*}[htbp!]
\centering
\includegraphics[width=0.495\textwidth]{FigS6a.pdf}
\includegraphics[width=0.495\textwidth]{FigS6b.pdf}
\caption{Time-evolution of the number of excess liquid-like molecules $\Delta n_l$ during the TIP4P/Ice crystallization simulations three replicas of the ice Ih basal (left panel) and prism1 (right panel) surfaces at 255 K. The piecewise linear fitting technique obtained the ice growth rate. The liquid-like molecules were evaluated using order parameter $lq_3$ at a threshold of -0.67.}
\label{255k}
\end{figure*}

\begin{figure*}[htbp!]
\centering
\includegraphics[width=0.495\textwidth]{FigS7a.pdf}
\includegraphics[width=0.495\textwidth]{FigS7b.pdf}
\caption{Time-evolution of the excess number of liquid-like molecules $\Delta n_l$ during the TIP4P/Ice crystallization simulations three replicas of the ice Ih basal (left panel) and prism1 (right panel) surfaces at 260 K. The piecewise linear fitting technique obtained the ice growth rate. The liquid-like molecules were evaluated using order parameter $lq_3$ at a threshold of -0.67.}
\label{260k}
\end{figure*}

\begin{figure*}[htbp!]
\centering
\includegraphics[width=0.495\textwidth]{FigS8a.pdf}
\includegraphics[width=0.495\textwidth]{FigS8b.pdf}
\caption{Time-evolution of the excess number of liquid-like molecules $\Delta n_l$ during the TIP4P/Ice crystallization simulations three replicas of the ice Ih basal (left panel) and prism1 (right panel) surfaces at 265 K. The piecewise linear fitting technique obtained the ice growth rate. The liquid-like molecules were evaluated using order parameter $lq_3$ at a threshold of -0.67.}
\label{265k}
\end{figure*}

\begin{figure*}[htbp!]
\centering
\includegraphics[width=0.495\textwidth]{FigS9a.pdf}
\includegraphics[width=0.495\textwidth]{FigS9b.pdf}
\caption{Time-evolution of the excess number of liquid-like molecules $\Delta n_l$ during the TIP4P/Ice crystallization simulations three replicas of the ice Ih basal (left panel) and two replicas of the prism1 (right panel) surfaces at 270 K. The piecewise linear fitting technique obtained the ice growth rate. Because there is a long time fluctuation at 270 temperature where there is a large float, some of the initial floating points have been omitted. Because there is a long period of data fluctuation at the beginning, some data points were omitted before fitting relative to other temperatures. The liquid-like molecules were evaluated using order parameter $lq_3$ at a threshold of -0.67.}
\label{270k}
\end{figure*}

\begin{figure*}[htbp!]
\centering
  \includegraphics[width=0.85\textwidth]{FigS10a.pdf}  
  \includegraphics[width=0.85\textwidth]{FigS10b.pdf}
  \caption{Time-evolution of the formation of the four ice bilayers (60-64 \AA, 64-68 \AA, 68-72 \AA, 72-76 \AA, corresponding to the bilayers from 1 to 4 along the model Z direction on the basal plane, respectively; 59-63 \AA, 63-67 \AA, 67-71 \AA, 71-75 \AA, corresponding to the bilayers from 1 to 4 along the model Y direction on the prism1 plane, respectively) above the interface where the melted area meets the area of ice on the basal (top panel) and prism1 (bottom panel) surfaces during the TIP4P/Ice crystallization process at 260 K. The darker blue indicates that the molecules are in a more ordered state, i.e., ice-like molecules; the more reddish molecules correspond to a more disordered state, i.e., liquid-like molecules. The oxygen atoms are coloured according to the values of the order parameter $lq_3$ with the threshold of -0.67.}
  \label{tip4p_kinetics}
\end{figure*}

\begin{figure*}[htbp!]
\centering
  \includegraphics[width=0.85\textwidth]{FigS11a.pdf}  
  \includegraphics[width=0.85\textwidth]{FigS11b.pdf}
  \caption{Time-evolution of the formation of the four ice bilayers above the interface where the melted area meets the ice region for the basal (top panel) and prism1 (bottom panel) surfaces during the TIP4P/Ice crystallization process at 265 K. The darker blue indicates that the molecules are in a more ordered state, i.e., ice-like molecules; the more reddish the dots are, the more disordered the molecules are, i.e., liquid-like molecules. The oxygen atoms are coloured according to the values of the order parameter $lq_3$ at the threshold of -0.67.}
  \label{tip4p_kinetics}
\end{figure*}

\begin{figure*}[htbp]
\centering
\includegraphics[width=1.0\textwidth]{FigS12.jpg}
\caption[The formation of the final layer tightly adhering the QLL on the basal and prism1 surfaces during the TIP4P/Ice crystallization process at 260 K.]{The formation of the final layer tightly adhering the QLL on the basal (top panel) and prism1 (bottom panel) surfaces during the TIP4P/Ice crystallization process at 260 K. Left panels: the number density profiles of the basal and prism1 surfaces before the final layer freezes and this moment is labelled as state A. Middle panels: The trajectory shows the evolution of the number of liquid-like molecules from the initial state A before the final layer freezes to the state B after complete freezing on the basal and prism1 surfaces. The liquid-like molecules were identified by the order parameter $lq_3$ coloured in red. Only oxygen atoms are shown. Right panels: the number density profiles of the basal and prism1 surfaces after the final layer completely freezes, and this moment is labelled as state B. These final layers in the figure for basal and prism1 surfaces at different states are labelled in the figure using the abbreviation FL.}
  \label{fig: final_layer}
\end{figure*}

\end{document}
